# Supplementary material for: Verti-Bench: A General and Scalable Off-Road Mobility Benchmark for Vertically Challenging Terrain
Source: arXiv:2502.11426 source file (2025-04-27)
Supplement: Supplementary file 1 [file appendix.tex]

\section*{Appendix}

All texture/semantics

All vehicle types
